# Supplementary material for: Fine-Tuning Automatic Speech Recognition for People with Parkinson's: An Effective Strategy for Enhancing Speech Technology Accessibility
Source: arXiv:2409.19818 source file (2024-09-29)
Supplement: Supplementary file 1 [file appendix.tex]

\begin{item}
\color{blue}
Some of the insisghts are \\
\begin{itemize}
    \item Fine-tuning on the Speech Accessibility corpus yields superior results compared to fine-tuning on LibriSpeech, showing a 25.43\% reduction in overall word error rate (WER). Yet 
    \item Two kinds of speaker clusters are formed according to speaker identification features and speech impairment severity levels, respectively.
    \item In contrast to what was observed with HMM-based speech recognizers \cite{7078583}, where systems trained on selected speakers based on speech closeness yielded significantly better results than using all speakers, our experiments demonstrate that using all speakers surpasses any single cluster we've created.
    \item K-means clustering of x-vectors, with the number of cluster set to two,  divides the corpus into genders with an accuracy rate near one hundred percent.
    \item Fine-tuning by gender yields more significant WER improvements for the targeted gender group, compared to the system fine-tuned on Librispeech 960h dataset. However, utilizing data from all speakers further improved both overall and gender-specific WER. Specaugmentation by gender does not benefit the WER.
    \item The severity levels are classified according to the average unit error rate (UER) of a speaker as determined by the system fine-tuned on Librispeech 960h dataset. Four severity levels—very low (VL), low (L), median (M), and high (H)—are determined by UER less than 10\%, 10\% to 20\%, 20\% to 40\%, and larger than 40\%, respectively.
    \item To conduct fine-tuning by severity experiments while ensuring comparable amount of training data, we first compare the models fine-tuned using the "VL", "L" and "M+H" classes. Among these, fine-tuning on the "L" class gives the best overall UER. Although the model fine-tuned using "VL" data achieves the best performances on the "VL" class correspondingly, it becomes increasingly less powerful in recognizing speech of higher severity levels. Furthermore, while the model fine-tuned on "M+H" is the least effective among the three models, it demonstrates significant overall improvements when "H" data is excluded, although the gap is narrowing as the severity level increases.
    \graphicspath{ {image/} }
        \begin{figure}
        	\centering
            \includegraphics[scale=0.35]{figures/Figure1.png}
        	\caption{relative UER improvements when fine-tuning by severity, n=1}
        	\label{FIG:1}
        \end{figure}
    \item As we enlarge training data by combining two of the three classes, namely "VL", "L", and "M+H", the overall performance improves. Specifically, the most effective model fine-tuned on "VL+L" gains an additional 8.75\% improvement in overall UER, compared to the model fine-tuned on "L". Again, compare the model fine-tuned on "L+M+H" and "L+M", excluding "H" data gives a 4.9\% relative UER improvement.
    \graphicspath{ {image/} }
        \begin{figure}
        	\centering
            \includegraphics[scale=0.35]{figures/Figure2.png}
        	\caption{relative UER improvements when fine-tuning by severity, n=2}
        	\label{FIG:2}
        \end{figure}
    \item Although combining all the data does not improve the overall UER over using "VL+L", there is a reduction in UER for both "M" and "H". When we exclude "H" from the training set, the best overall UER achieved, as well as the UER of the "H" class.
    \graphicspath{ {image/} }
        \begin{figure}
        	\centering
            \includegraphics[scale=0.35]{figures/Figure3.png}
        	\caption{relative UER improvements when fine-tuning by severity, n=3}
        	\label{FIG:3}
        \end{figure}

    \graphicspath{ {image/} }
        \begin{figure}
        	\centering
            \includegraphics[scale=0.35]{figures/Figure4.png}
        	\caption{relative UER improvements of best performing models fine-tuned by severity, n=1, 2, 3}
        	\label{FIG:4}
        \end{figure}

    \item The WER analysis gives different results.
    \item To conduct fine-tuning by severity experiments while ensuring comparable amount of training data, we first compare the models fine-tuned using the "VL", "L" and "M+H" classes. Among these, fine-tuning on the "L" class gives the best overall UER. Although the model fine-tuned using "VL" data achieves the best performances on the "VL" class correspondingly, it becomes increasingly less powerful in recognizing speech of higher severity levels. Furthermore, while the model fine-tuned on "M+H" is the least effective among the three models, it demonstrates significant overall improvements when "H" data is excluded, although the gap is narrowing as the severity level increases.
    \graphicspath{ {image/} }
        \begin{figure}
        	\centering
            \includegraphics[scale=0.35]{figures/Figure1.png}
        	\caption{relative UER improvements when fine-tuning by severity, n=1}
        	\label{FIG:1}
        \end{figure}
    \item As we enlarge training data by combining two of the three classes, namely "VL", "L", and "M+H", the overall performance improves. Specifically, the most effective model fine-tuned on "VL+L" gains an additional 8.75\% improvement in overall UER, compared to the model fine-tuned on "L". Again, compare the model fine-tuned on "L+M+H" and "L+M", excluding "H" data gives a 4.9\% relative UER improvement.
    \graphicspath{ {image/} }
        \begin{figure}
        	\centering
            \includegraphics[scale=0.35]{figures/Figure2.png}
        	\caption{relative UER improvements when fine-tuning by severity, n=2}
        	\label{FIG:2}
        \end{figure}
    \item Although combining all the data does not improve the overall UER over using "VL+L", there is a reduction in UER for both "M" and "H". When we exclude "H" from the training set, the best overall UER achieved, as well as the UER of the "H" class.
        
\end{itemize}
\end{item}

The table of results is linked here.\\
\url{https://docs.google.com/spreadsheets/d/19SkKk4GD_kbnR7l0rN7b4ZCcOMorgedkwTKw6xiSq5E/edit#gid=1570910768}
